# Supplementary material for: The observation of quantum fluctuations in a kagome Heisenberg antiferromagnet
Source: arXiv:2210.12627 source file (2022-10-23)
Supplement: Supplementary file 1 [file Supplementary_r2.pdf]

*Supplementary Information*

## The observation of quantum fluctuations in a kagome Heisenberg antiferromagnet

Fangjun Lu, Long Yuan, Jian Zhang, Boqiang Li, Yongkang Luo, and Yuesheng Li

### Supplementary Note 1. Refinement of the random exchange Hamiltonian

The previously reported crystal structure determined by single-crystal XRD and density functional theory (DFT) calculation with a Coulomb repulsion ($U$) has revealed that the inherent antisite disorder of polar $OH2^-$ and nonpolar $Br2^-$ pushes 70(2)% of $Y^{3+}$ away from its ideal position by a distance of $\Delta z_{\mathrm{Y2}} \sim \pm 0.7$Å and this influences the nearest-neighbor (NN) exchange couplings ($J_1$) of the kagome Heisenberg antiferromagnet (KHA) YCOB [1]. The nonsymmetric local environments of $OH2^-$/$Br2^-$ give rise to hexagons with alternate exchanges ($J_{\mathrm{1a}}$ and $J_{\mathrm{1c}}$) on the kagome lattice, whereas the rest symmetric stacking sequences of $OH2^-$/$Br2^-$ result in almost uniform hexagons ($J_{\mathrm{1b}}$), as illustrated in Supplementary Fig. 2a. The DFT+$U$ calculations suggest that both further-neighbor and interlayer exchange couplings are less than 4% of $\langle J_1 \rangle$ [1], due to the spatial localization of the $3d$ electrons in the insulating YCOB. The measured magnetic anisotropy, $\chi_{\|}/\chi_{\perp}$, only increases by $\sim$ 4% from $T$ = $\langle J_1 \rangle$ down to 1.8 K $\sim$ 0.03$\langle J_1 \rangle$ [1], suggesting that the interaction anisotropy is not critical due to the weak spin-orbit coupling of the $3d$ electrons.

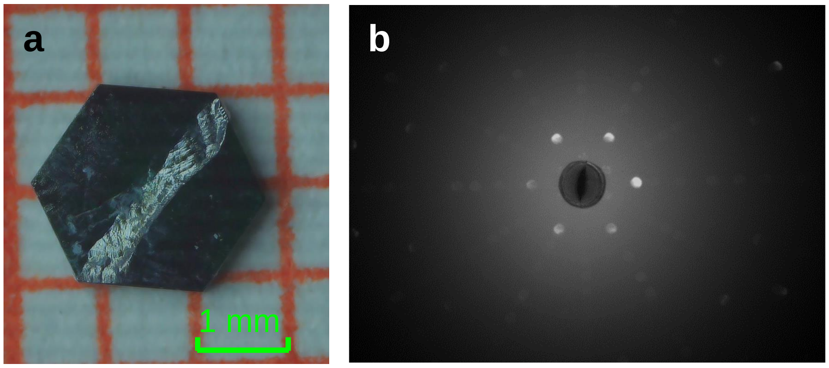


**Supplementary Figure 1. Single crystal used in NMR measurements.** (**a**) The single crystal ($S_1$) of $YCu_3(OH)_{6.5}Br_{2.5}$ (YCOB) used in NMR measurements. (**b**) Laue x-ray diffraction (XRD) pattern measured on the $ab$ plane, i.e., the largest surface of the single crystal shown in **a**.

Analogous to the simplified crystal structure of YCOB [2] with three discrete Y positions, $\Delta z_{\mathrm{Y1}}$ = 0 and $\Delta z_{\mathrm{Y2}} \sim \pm 0.7$Å, we constructed a similarly simplified random exchange model with three discrete couplings, $J_{\mathrm{1a}}$, $J_{\mathrm{1b}}$, and $J_{\mathrm{1c}}$, on the kagome lattice (Supplementary Fig. 2a). The real situation might be much more complicated, but we seek to explain the experimental observations within a minimum model that

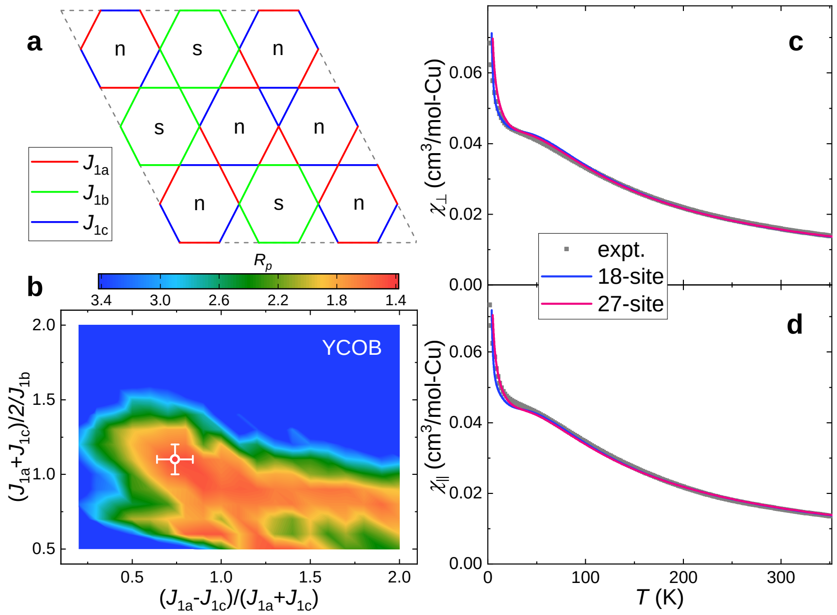


**Supplementary Figure 2. Refinement of the exchange Hamiltonian.** (**a**) Sketch of a random KHA sample with $1 - f_{\mathrm{Y1}} \sim 0.7$ of randomly distributed nonsymmetric (n) hexagons of alternate exchanges (blue and red) and the rest of symmetric (s) hexagons (green). (**b**) The deviation $R_p$[a] obtained by fitting the magnetic susceptibilities with fixed occupancy $f_{\mathrm{Y1}}$ = 0.3 (experimentally determined by single-crystal XRD). The magnetic susceptibilities of YCOB measured at 1 T are shown in panels **c** and **d**, for field applied along the $ab$ plane and $c$ axis, respectively. The colored lines show the FTLD susceptibilities calculated on the 18- and 27-site clusters with periodic boundary conditions, using $J_{1a}$ = 89.4 K, $J_{1b}$ = 47.9 K, and $J_{1c}$ = 15.8 K.

[a] $R_p = \sqrt{\frac{1}{N_0}\sum_i(\frac{X_i^{\mathrm{obs}}-X_i^{\mathrm{cal}}}{\sigma_i^{\mathrm{obs}}})^2}$, where $N_0$, $X_i^{\mathrm{obs}}$ and $\sigma_i^{\mathrm{obs}}$ are the number of the data points, the observed value and its standard deviation, respectively, whereas $X_i^{\mathrm{cal}}$ is the calculated value.

captures the essential physics. The observables calculated by the 18- and 27-site finite-temperature Lanczos diagonalization (FTLD) are evaluated over 80 and 30 independent samples, respectively. For the simulation of the dynamic spin-lattice relaxation rate ($1/T_1$), more than 100 Lanczos steps are typically required. From fitting the magnetic susceptibilities above 6 K $\sim 0.1\langle J_1\rangle$ (see Supplementary Fig. 2c,d), we obtain $J_{1a}$ = 89 K, $J_{1b}$ = 48 K, and $J_{1c}$ = 16 K with the least $R_p$ = 1.4(1). The resulted $(J_{1a} - J_{1c})/(J_{1a} + J_{1c})$ = 0.7(1), $(J_{1a} + J_{1c})/(2J_{1b})$ = 1.1(1), and $\langle J_1\rangle = 0.35J_{1a} + 0.3J_{1b} + 0.35J_{1c} \sim 51$ K are well consistent with the previously reported result [1] (Supplementary Fig. 2b). Furthermore, the resulted $R_p$ = 1.4(1) is very close to the lower limit $R_p \sim 1$, and the finite-size effect of the FTLD calculation is negligible above $T \sim 0.1\langle J_1\rangle$ (see Supplementary Fig. 2c,d), proving the validity of this random exchange model.

Due to the inherent exchange randomness, different bricks of spins ($S_i$) on the kagome lattice of YCOB have different local magnetization at a magnetic field and low temperatures, $\langle S^z\rangle$ = $\sum_{i\in\text{brick}}\langle S_i^z\rangle/N_{\text{brick}}$, where $N_{\text{brick}}$ = 3 or 6 is the number of spins in each triangular or hexagonal brick, respectively, and $\langle S_i^z\rangle$ = $\sum_m \mathrm{e}^{-\frac{E_m}{k_\mathrm{B}T}}\langle m|S_i^z|m\rangle/\sum_m \mathrm{e}^{-\frac{E_m}{k_\mathrm{B}T}}$. In our 27-site FTLD calculation, 30 independent samples are taken into account to simulate the effect of quenched randomness, and thus there are 27×30 = 810 spins, 810×2/3 = 540 triangles, 810/3×0.7 = 189 nonsymmetric hexagons, and 810/3×0.3 = 81 symmetric hexagons. Therefore, one can define the distributed density function, d$n_S(\langle S^z\rangle)$/d$\langle S^z\rangle$, which depends on $T$ and accounts for the broadening of the NMR main lines. Here, d$n_S(\langle S^z\rangle)$ is the number of bricks with the local magnetization (per site) ranging from $\langle S^z\rangle$ to $\langle S^z\rangle$+d$\langle S^z\rangle$.

## Supplementary Note 2. Identification of $^{81}$Br and $^{79}$Br NMR

Because the gyromagnetic ratio of $^{63}$Cu ($^{63}\gamma_\mathrm{n}$ = 11.285 MHz/T) and $^{81}$Br ($^{81}\gamma_\mathrm{n}$ = 11.4989 MHz/T) are close, the $^{63}$Cu signal from the copper coil can be regarded as the hallmark of these measurements. Supplementary Fig. 3a displays a representative spectrum taken at $T$ = 265 K and $\mu_0H_{||}\sim$ 10.75 T. Three peaks can be seen in the frequency window 121-125 MHz. The sharp peak centered at 121.632 MHz has a full width at half maximum (FWHM) only ∼10 kHz, it, therefore, is reasonable to ascribe it as $^{63}$Cu in coil. This leads to a precise magnetic field value $\mu_0H_{||}$ = 10.7525 T with the Knight shift of elemental Cu $K$ = 0.2394% already known [3]. The two other peaks near 123.41 MHz and 123.84 MHz can not originate from $^{63}$Cu in YCOB, because they disappear when we attempted to detect them in the $^{65}$Cu measurements (cf the red curve in Supplementary Fig. 3b), but instead they show up in the $^{79}$Br measurements under $\mu_0H_{||}$ = 11.5870 T. The NMR shifts of Br2 and Br1 determined from $^{79}$Br and $^{81}$Br are in good agreement. Furthermore, the weight ratio between these two peaks is $I_{\text{Br2}}/I_{\text{Br1}}\sim$ 0.2, close to the stoichiometric ratio of Br2 and Br1 determined by single-crystal XRD (see inset of Fig. 2b in main text), and this provides additional evidence that the two peaks respectively stem from Br2 and Br1 sites in YCOB. Note that no satellite transitions arising from nuclear quadruple effect related to $^{81}$Br (nuclear spin $I$ = 3/2) can be resolved in this frequency range. The missing of $^{63}$Cu signal from YCOB is probably due to a large NMR shift (thus is moved out from the detected frequency range) or a very short spin-spin relaxation time ($T_2$ wipe-out), and further measurements are required to clarify this issue.

## Supplementary Note 3. Br1 nuclear spin-lattice and spin-spin relaxation

Spin-lattice relaxation rate ($1/T_1$) of Br1 was measured by the inversion recovery method whose pulse sequence is depicted in the inset of Fig. 4a in the main text. The $T_1$ relaxation data can be fitted to a

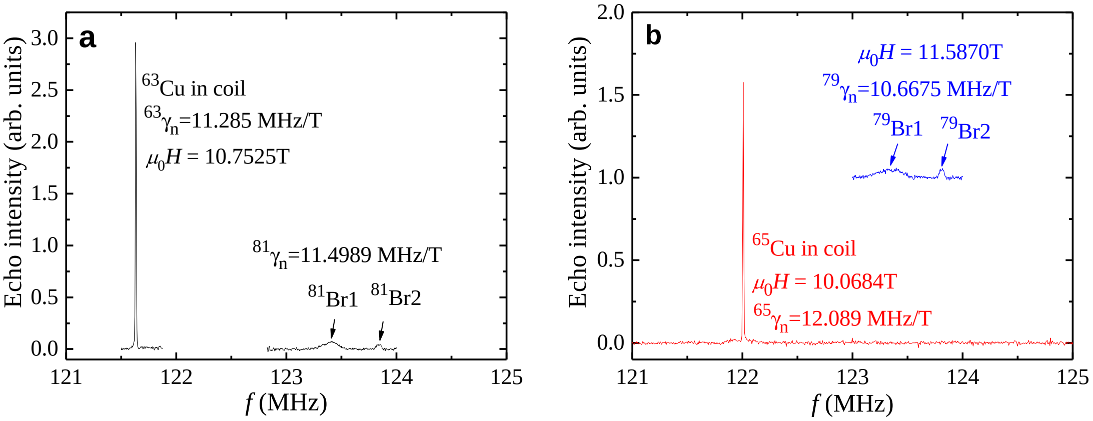


**Supplementary Figure 3. Frequency sweep spectra (121-125 MHz) taken at 265 K.** (**a**) At $\mu_0 H_{||}$ = 10.7525 T, one sees three peaks arising from $^{63}$Cu in coil, $^{81}$Br1 and $^{81}$Br2 in YCOB sample, respectively. (**b**) Red curve, at $\mu_0 H_{||}$ = 10.0684 T, only one sharp peak is resolved, from $^{65}$Cu in coil. Blue curve, at $\mu_0 H_{||}$ = 11.5870 T, two relatively broader peaks can be seen which are attributed to $^{79}$Br of the sample. The base line of the blue curve has been shifted vertically for clarity.

stretched-exponential function for the central transition of $I$ = 3/2 nuclear spins, i.e.,

$$M(t)|_{-\frac{1}{2}\leftrightarrow\frac{1}{2}} = M_0 - 2M_0 F\{\frac{1}{10}\exp[-(\frac{t}{T_1})^{\beta}] + \frac{9}{10}\exp[-(\frac{6t}{T_1})^{\beta}]\}. \quad (1)$$

When the stretching exponent is fixed to $\beta$ = 1, Supplementary equation (1) gets back to the standard formula. From fitting the data measured at 2.8 K (< 15 K), we find that including the additional fitting parameter $\beta$ only slightly increases the adj. $R^2$ [4] from 0.9975 (at $\beta$ = 1) to 0.9982 (at $\beta$ = 0.83), and the fitted $\beta$ = 0.83(9) is much larger than $\sim$ 1/3 expected for a conventional spin-glass freezing [5]. Our experimental observations suggest the $T_1$ relaxation is not strongly stretched even at low temperatures.

Spin-spin relaxation rate ($1/T_2$) of Br1 was measured by the Hahn spin-echo decay method, the pulse sequence of which is sketched on the top of Supplementary Fig. 4. A representative result of 8 K is shown in Supplementary Fig. 4 as an example. The spin-echo intensity $M(2t)$ decreases with the increasing time interval between the $\pi/2$ and $\pi$ pulses, following the exponential function:

$$M(2t) = M_0 \exp(-2t/T_2). \quad (2)$$

This fitting yields $T_2$ = 48(1) $\mu$s for $T$ = 8 K.

**Supplementary Note 4. Low-$T$ NMR spectra measured with different delays of the spin-echo sequences**

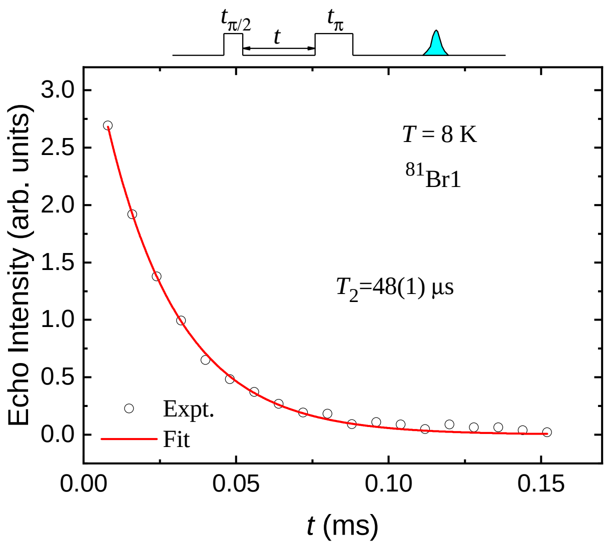


**Supplementary Figure 4. Nuclear spin-spin relaxation.** A selected $T$ = 8 K spin-spin relaxation of Br1 measured by Hahn spin-echo decay method, fitted to Supplementary equation (2). The symbols denote the experimental results, while the red lines are the fitting curves. The pulse sequence for $T_2$ measurements in depicted on the top of the figure.

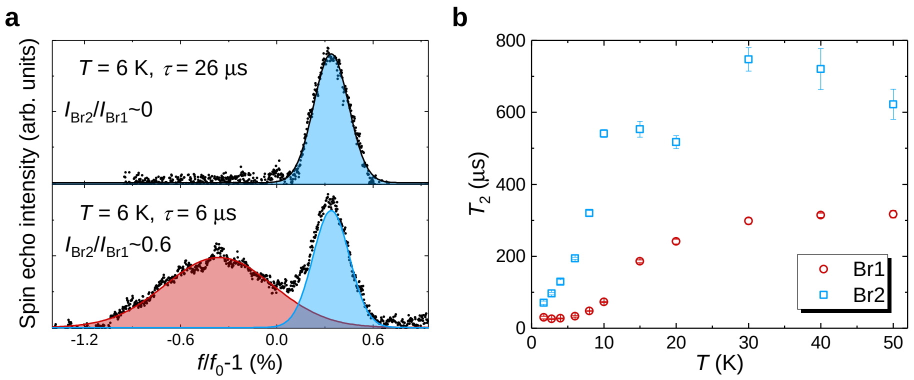


**Supplementary Figure 5. NMR spectra and transverse relaxation times.** (**a**) Frequency-sweep NMR spectra of YCOB measured with different delays $\tau$ of the spin-echo sequences at 6 K. (**b**) Temperature dependence of transverse relaxation times $T_2$(Br1) and $T_2$(Br2).

Supplementary Fig. 5a shows the NMR spectra measured with different delays $\tau$ of the spin-echo sequences, at the same low temperature of 6 K ($<$ 15 K). When a typical $\tau$ of 26 $\mu$s is used, the broader NMR line from Br1 nuclear spins disappears at low temperatures, due to the short transverse relaxation time $T_2$(Br1) of 33(2) $\mu$s (Supplementary Fig. 5b) that is compatible with $\tau$. In contrast, when using the shortest

delay $\tau$ = 6 $\mu$s of our setup the situation gets much better and the Br1 NMR line appears again. However, the ratio between the *integrated* intensities, $I_{\mathrm{Br2}}/I_{\mathrm{Br1}}$, sharply increases to $\sim$ 0.6 below 15 K (please see the inset of Fig. 2b of the main text), and thus the overall intensity of the Br1 NMR line is still significantly suppressed due to the short $T_2$(Br1), which is still compatible with $\tau$ = 6 $\mu$s. For the Br2 NMR line the suppression of the intensity is less apparent, because $T_2$(Br2) is about two times larger than $T_2$(Br1) in the full temperature range, which is another strong signature of different origins of the Br1 and Br2 NMR lines.

**Supplementary Note 5. Absence of conventional spin freezing**

Glassy freezing/dynamics is typically observed by NMR as a broad peak in the nuclear spin-lattice relaxation rate 1/$T_1$ vs temperature $T$ when the inverse correlation time matches the NMR frequency, and such a peak ($T_1$ minimum) defines the freezing temperature $T_c$ [6–8]. Moreover, 1/$T_1$ is usually expected to increase by more than one order of magnitude at $T_c$ from that above $T_c$, as reported in refs [6–8] for example. However, such a robust peak in 1/$T_1$ vs $T$ is absent in YCOB, as shown in Supplementary Fig. 6a. Therefore, conventional spin-glass freezing between 1.7 and 300 K should be precluded. Furthermore, both ac and dc susceptibilities also do not exhibit any peak features (see Supplementary Fig. 6d,e). Neither obvious frequency dependence of ac susceptibilities nor splitting of ZFC and FC dc susceptibilities was observed [1, 2, 9], confirming the absence of any conventional spin-glass freezing down to 1.8 K in YCOB.

Neither 1/$T_1$ nor 1/$T_2$ of YCOB shows any conventional critical enhancement (peak) in their temperature dependence (see Supplementary Fig. 6), which speaks against the presence of conventional spin freezing at $T \geq$ 1.7 K $\sim 0.03\langle J_1\rangle$. Moreover, as reported in our previous bulk study the residual magnetic entropy of YCOB obtained from the specific heat gets small below 1.7 K, $S_m \leq 3.4\%R$ln2 [1], suggesting the approaching of ground-state properties. These observations consistently suggests that the majority of spins remain disordered at low temperatures.

Of course, the enhancement of the 1/$T_1$ and 1/$T_2$ at low $T$ indeed indicate the slowing down of spin fluctuations parallel and perpendicular to the kagome lattice of YCOB, respectively, at $H \parallel c$. However, even in the fully frustrated and disorder-free case, the slowing down of spin fluctuations is also expected in the quantum spin liquid (QSL) phase at low $T$, as the thermal fluctuations must be dramatically suppressed by cooling. In following paragraphs, we compare the main features of our NMR results measured on YCOB with those of other well-studied QSL candidates.

(1) The spin-lattice relaxation rate of YCOB only slightly increases by less than two times as the temperature decreases from $\sim$ 300 K down to 1.7 K (Supplementary Fig. 6a), which suggests the survival of strong quantum fluctuations along the kagome lattice, $\sim$ 70% of the total spin fluctuations seen at high $T$ [10]. This feature is consistent with the expectation of the gapless (spin gap $<$ 1.7 K $\sim 0.03\langle J_1\rangle$) QSL

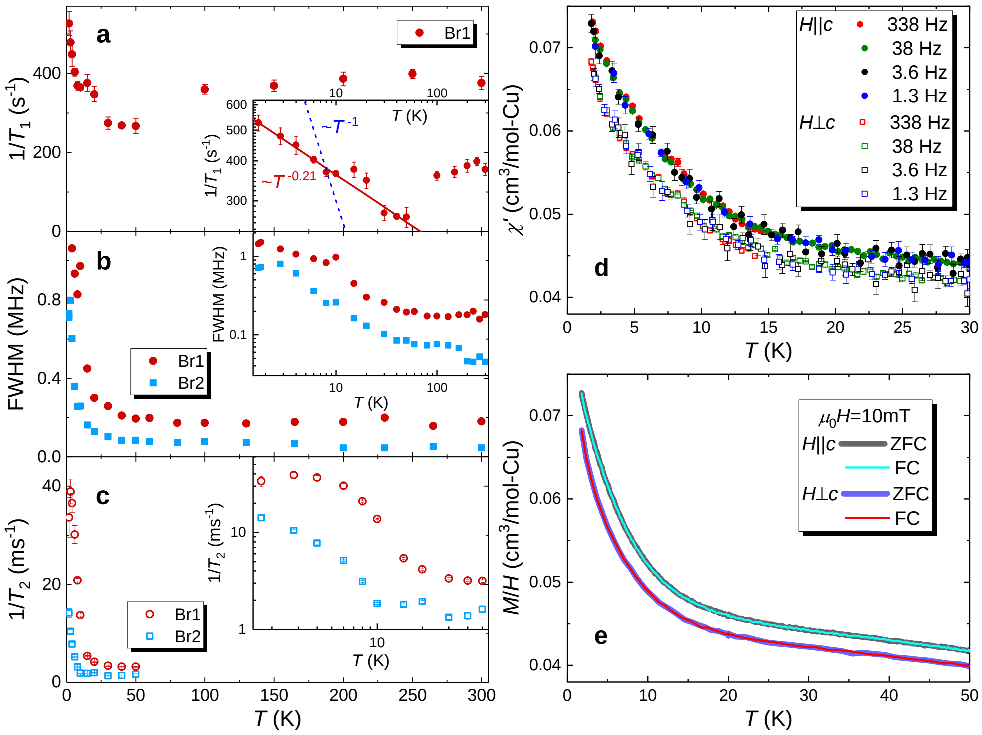


**Supplementary Figure 6. Temperature evolution of NMR quantities and bulk susceptibilities.** Temperature dependence of spin-lattice relaxation rates ($1/T_1$, **a**), full widths at half maximum (FWHMs) of the main NMR lines (**b**), and spin-spin relaxation rates ($1/T_2$, **c**). The insets of **a**-**c** present the log-log plots of the corresponding data. In the inset of **a**, the solid line displays the power-law fit, $1/T_1 \sim T^{-0.21(1)}$, whereas the dashed line shows a slowing down of thermal/classical fluctuations, $1/T_1 \sim T^{-1}$, for comparison. (**d**) ac susceptibilities (real parts) measured by applying ac magnetic fields with various frequencies and the fixed amplitude of 1 mT, parallel and perpendicular to the $c$ axis. (**e**) dc susceptibilities measured at 10 mT under zero-field cooling (ZFC) and field cooling (FC), respectively. The data of **d** and **e** are abstracted from ref. [1].

phase either with or without nodes [11]. Upon cooling, the similar increase of low-$T$ $1/T_1$ was also observed in the triangular-lattice QSL candidates $EtMe_3Sb[Pd(dmit)_2]_2$ [11] and $Na_2BaCo(PO_4)_2$ below 2 T [12], the three-dimensional candidate $PbCuTe_2O_6$ below $\sim$ 2 K [13], etc.

(2) The FWHMs of the Br1 and Br2 NMR lines increase by $\sim$ 5 and 10 times, respectively, as the temperature decreases from $\sim$ 300 K down to 1.7 K in YCOB (Supplementary Fig. 6b). Similarly, in the well-known kagome-lattice QSL candidate $ZnCu_3(OH)_6Cl_2$ FWHMs also increase by $\sim$ 10 times from $\sim$ 120 K down to the lowest temperature [14]. The similar inhomogeneous broadening of NMR lines was also observed in the triangular-lattice QSL candidates $EtMe_3Sb[Pd(dmit)_2]_2$ [11] and $\kappa$-$(ET)_2Cu_2(CN)_3$ [15].

(3) The enhancement of $1/T_2$ (Supplementary Fig. 6c) at low $T$ is also very common among QSL candidates, as reported in refs [13, 15, 16] for instance.

In summary, our NMR results (including $1/T_1$, FWHM, and $1/T_2$) of YCOB are well consistent with the previously reported ac and dc susceptibilities [1, 2, 9] and exhibit the common features of well-studied QSL candidates, and speak against a critical slowing down or critical broadening of conventional spin-glass freezing at least down to 1.7 K. No well-defined critical temperature, such as $T_c$ where $1/T_1$ shows a robust peak, can be abstracted from the NMR quantities vs $T$ plots (see Supplementary Fig. 6a-c).

**Supplementary Note 6. Negligible second-order quadrupole shifts of the main NMR lines**

Both $^{81}$Br and $^{79}$Br have large quadrupole moments, but the quadrupole shifts of both Br1 and Br2 main lines are symmetrically forbidden in our NMR measurements on YCOB. Both point groups on Br1 and Br2 positions contain the three-fold rotational symmetry on the $c$ $(z)$ axis $R_3^z$, and thus the general electric field gradient (EFG) tensor that is invariant under $R_3^z$ is given by

$$\boldsymbol{V} = \begin{pmatrix} V_{xx} & 0 & 0 \\ 0 & V_{xx} & 0 \\ 0 & 0 & V_{zz} \end{pmatrix}. \tag{3}$$

There are only two parameters $V_{xx}$ and $V_{zz}$ that depend on the distinctive Wyckoff positions, $2d$ (Br1) and $1a$ (Br2). As long as $|V_{zz}| > |V_{xx}|$ is satisfied, the second-order quadrupole shift of the main line is symmetrically forbidden in our experiments. As shown in the main text the measured NMR shifts of Br1 and Br2 lines can be naturally understood by the ab-initio many-body simulation without any quadrupole corrections, and of course this is a strong signature of the absence of profound quadrupole shifts at the main lines.

To clear the doubt away, we conducted the DFT calculation of the EFG tensors at Br1 and Br2 sites by considering the possible misalignment of the crystal and structural disorder. We started with several optimized crystal structures for supercells containing different environments of Br/OH, and then calculated the EFG tensors at various Br1 and Br2 sites. Typical EFG tensors at Br1 and Br2 sites are obtained,

$$\boldsymbol{V}(\mathrm{Br1}) = \begin{pmatrix} -35.746 & 0.282 & 0.390 \\ 0.282 & -36.057 & 0.283 \\ 0.390 & 0.283 & 71.803 \end{pmatrix}, \boldsymbol{V}(\mathrm{Br2}) = \begin{pmatrix} -48.510 & 0.029 & 0.080 \\ 0.029 & -48.491 & 0.019 \\ 0.080 & 0.019 & 97.001 \end{pmatrix}, \tag{4}$$

in V/Å$^2$. Obviously, all of the calculated EFG tensors with the quenched structural disorder are very close to the general form presented in Supplementary equation (3) with $|V_{zz}| > |V_{xx}|$.

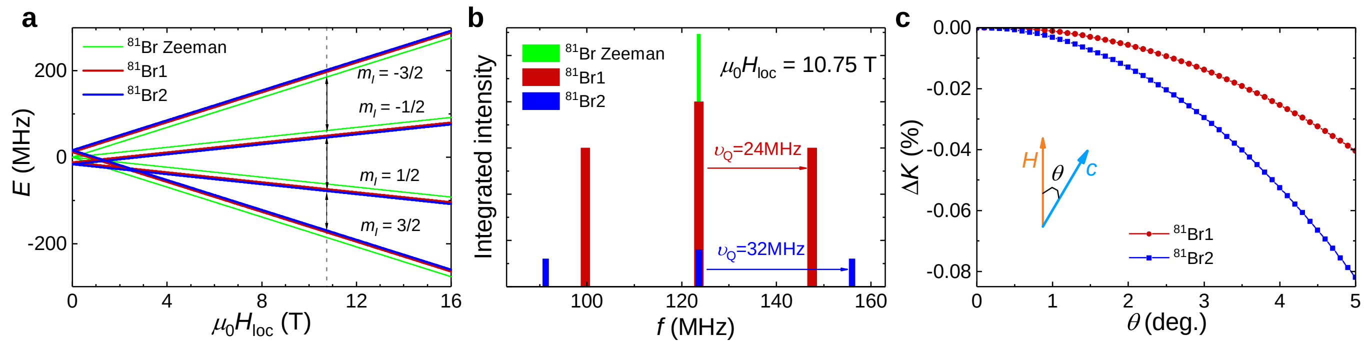


**Supplementary Figure 7. Simulations of the quadrupole effects.** (**a**) The field dependence of eigenvalues of Supplementary equation (5) calculated for $\boldsymbol{V}(\mathrm{Br1})$ and $\boldsymbol{V}(\mathrm{Br2})$. (**b**) The NMR spectra at $\mu_0 H_{\mathrm{loc}}$ = 10.75 T. Nearly zero quadrupole correction (shift) of the main peak is observed, and two satellite lines are well separated from the main one by the nuclear quadrupole frequency $\nu_Q > 20$ MHz. (**c**) The misalignment angle ($\theta$) dependence of quadrupole corrections calculated for $\boldsymbol{V}(\mathrm{Br1})$ and $\boldsymbol{V}(\mathrm{Br2})$. $\theta$ is the possible small angle between the $c$ axis and applied magnetic field, as shown in the inset.

Under the local magnetic field of $\mu_0 H_{\mathrm{loc}}$ applied along the $c$ ($z$) axis, the total Hamiltonian (in Hz) as the sum of the Zeeman (dipole) and quadrupole terms is given by

$$\mathcal{H}_{\mathrm{NMR}} = -\mu_0 H_{\mathrm{loc}} \gamma_{\mathrm{n}} I_z + \frac{eQ}{2I(2I-1)h} \boldsymbol{I} \cdot \boldsymbol{V} \cdot \boldsymbol{I}^T, \tag{5}$$

where $\boldsymbol{I} = [I_x, I_y, I_z]$, $I$ = 3/2, $\gamma_{\mathrm{n}}$ = 11.4989 and 10.6675 MHz/T, $Q$ = 0.276 and 0.330 $\times 10^{-28}\mathrm{m}^2$, for $^{81}$Br and $^{79}$Br nuclear spins, respectively. The Hamiltonian of Supplementary equation (5) can be diagonalized exactly, the eigenvalues $E_n$ and integrated intensities proportional to $|\langle E_{n'}|I_x|E_n\rangle|^2$ can be obtained, as shown in Supplementary Fig. 7a,b for $\boldsymbol{V}(\mathrm{Br1})$ and $\boldsymbol{V}(\mathrm{Br2})$. The three lines of the NMR spectrum are well separated by the nuclear quadrupole frequency $\nu_Q = \frac{3eQ\tilde{V}_{zz}}{2I(2I-1)h} > 20$ MHz, where $\tilde{V}_{zz}$ is the largest absolute eigenvalue of $\boldsymbol{V}$. As a result, we only observed the main Br NMR lines of YCOB in our frequency range (see main text), and the second-order quadrupole shifts of the main lines are essentially negligible even in the presence of the inherent disorder, $|\Delta K| < 10^{-6}$.

We used the high-quality single crystals of YCOB on perfect flaky shape, and mounted the crystal sheets perpendicular to the applied magnetic field, i.e. $c \parallel H$, with carefulness. As a result, we found the misalignment angle ($\theta$) is typically very small based on Laue x-ray diffraction, saying $\theta < 5°$. The rotation

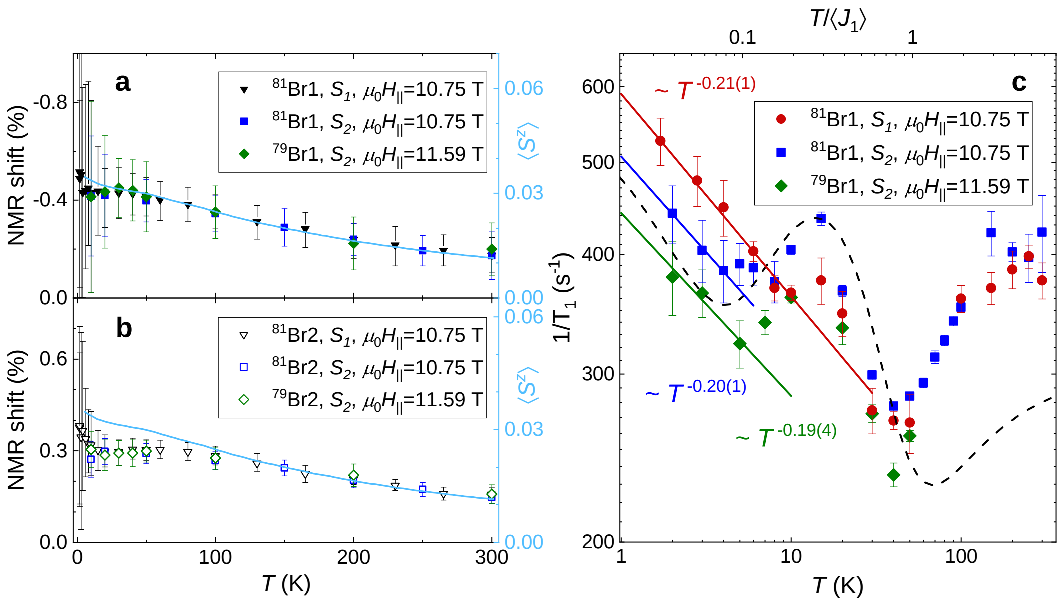


**Supplementary Figure 8. Weak sample dependence of NMR shifts and spin-lattice relaxation rates.** Temperature dependence of the main NMR shifts of Br1 (**a**) and Br2 (**b**) nuclear spins, with the bulk magnetization ($\langle S^z \rangle$) measured at $\mu_0 H_{||}$ = 10.75 T for comparison. The bars display the normalized frequency regions where the intensity is larger than half of the maximum value. (**c**) Temperature dependence of Br1 nuclear spin-lattice relaxation rates $1/T_1$. The colored lines present the power-law fits to the experimental data below 10 K, and the dashed line shows $1/T_1$ calculated by using the random KHA model of YCOB.

matrix is given by

$$\boldsymbol{R}(\theta,\varphi) = \begin{pmatrix} \cos\theta + (1-\cos\theta)\cos^2\varphi & (1-\cos\theta)\sin\varphi\cos\varphi & \sin\theta\sin\varphi \\ (1-\cos\theta)\sin\varphi\cos\varphi & \cos\theta + (1-\cos\theta)\sin^2\varphi & -\sin\theta\cos\varphi \\ -\sin\theta\sin\varphi & \sin\theta\cos\varphi & \cos\theta \end{pmatrix}, \quad (6)$$

where $0 \le \varphi < 360°$. By replacing $\boldsymbol{V}$ with $\boldsymbol{R}(\theta,\varphi)^{-1} \cdot \boldsymbol{V} \cdot \boldsymbol{R}(\theta,\varphi)$ in Supplementary equation (5), we calculated the quadrupole shift of main line $\Delta K$ (see Supplementary Fig. 7c), which is nearly independent of $\varphi$ due to $\tilde{V}_{yy} \approx \tilde{V}_{xx}$. Even when a misalignment of $\theta < 5°$ is taken into account, the quadrupole shifts of main lines are still negligible, $|\Delta K| < 0.08\%$, much smaller than the measured Knight shifts and line widths. Since the second-order quadrupole shifts of main NMR lines are symmetrically forbidden by $R_3^z$, the zero shift can act as the reference in our NMR measurements on the single crystal of YCOB with $c \parallel H$.

The Br1 ($2d$) and Br2 ($1a$) sites are symmetrically different with profoundly different distances and hyperfine paths to the electronic spin of magnetic $Cu^{2+}$, |Br1$-$Cu| = 2.88 Å and |Br2$-$Cu| = 4.49 Å, which

should account for the observed large difference of the hyperfine couplings, $A_{\rm hf1}$ = $-0.68(2)$ T/$\mu_{\rm B}$ and $A_{\rm hf2}$ = 0.55(3) T/$\mu_{\rm B}$ at Br1 and Br2 sites, respectively, in the absence of the second-order quadrupole shifts. It is difficult to reproduce these hyperfine couplings by first-principles calculations, due to the complicated underlying mechanism including both the positive and negative contributions.

As shown by the ab-initio many-body simulations (see the main text) the local spin susceptibilities at Br1 and Br2 sites, $\chi_{\rm loc}$(Br1) and $\chi_{\rm loc}$(Br2), are distinguishable only at low temperatures ($T < 100$ K). However, above 100 K $> \langle J_1 \rangle$ the spin susceptibilities get nearly homogeneous as evidenced by the minimal widths of the main NMR lines (Supplementary Fig. 6b), the difference between the calculated $\chi_{\rm loc}$(Br1) and $\chi_{\rm loc}$(Br2) is much smaller than the observed standard deviation of Knight shifts (see Fig. 3a in the main text), and thus the equation $K$ = $A_{\rm hf}\chi_{\rm loc}$+$K_0$ with $\chi_{\rm loc}$(Br1) $\approx$ $\chi_{\rm loc}$(Br2) $\approx$ $\chi_{\rm bulk}$ holds very well. As a result, we are able to obtain the precise hperfine couplings of Br1 and Br2 separately, by using the same bulk susceptibility ($\chi_{\rm bulk}$) measured by VSM, above 100 K (see inset of Fig. 2c in the main text).

To test the repeatability of the above results, we performed the independent NMR measurements on another single-crystal sample $S_2$ ($\sim$ 15.2 mg) that most likely has a different small misalignment angle $\theta$, but no essential difference from that measured on $S_1$ was found. The main shifts and 1/$T_1$ from both $^{81}$Br and $^{79}$Br nuclear spins measured on $S_2$ are shown in Supplementary Fig. 8, with comparison to the $^{81}$Br NMR results measured on $S_1$. The profiles of the NMR spectra measured at $^{81}$Br and $^{79}$Br frequencies are highly consistent with each other (see Supplementary Fig. 3), and the different hyperfine couplings measured at Br1 ($A_{\rm hf1}$ = $-0.68(2)$ T/$\mu_{\rm B}$) and Br2 ($A_{\rm hf2}$ = 0.55(3) T/$\mu_{\rm B}$) lines are confirmed by the $T$ dependence of both $^{81}$Br and $^{79}$Br NMR shifts measured on $S_2$ (see Supplementary Fig. 8a,b).

**Supplementary References**


[1] J. Liu, L. Yuan, X. Li, B. Li, K. Zhao, H. Liao, and Y. Li, "Gapless spin liquid behavior in a kagome Heisenberg antiferromagnet with randomly distributed hexagons of alternate bonds," Phys. Rev. B **105**, 024418 (2022).

[2] X.-H. Chen, Y.-X. Huang, Y. Pan, and J.-X. Mi, "Quantum spin liquid candidate $YCu_3(OH)_6Br_2[Br_x(OH)_{1-x}]$ ($x \approx 0.51$): With an almost perfect kagomé layer," J. Magn. Magn. Mater. **512**, 167066 (2020).

[3] G. C. Carter, L. H. Bennett, and D. J. Kahan, *Metallic shifts in NMR: A review of the theory and comprehensive critical data compilation of metallic materials. Progress in Materials Science* (Pergamon Press, 1976).

[4] See https://www.originlab.com/doc/Origin-Help/Interpret-Regression-Result for adj. $R^2$.

[5] A. T. Ogielski, "Dynamics of three-dimensional Ising spin glasses in thermal equilibrium," Phys. Rev. B **32**, 7384–7398 (1985).

[6] M.-H. Julien, F. Borsa, P. Carretta, M. Horvatić, C. Berthier, and C. T. Lin, "Charge segregation, cluster spin glass, and superconductivity in $La_{1.94}Sr_{0.06}CuO_4$," Phys. Rev. Lett. **83**, 604–607 (1999).

[7] X. Zong, A. Niazi, F. Borsa, X. Ma, and D. C. Johnston, "Structure, magnetization, and NMR studies of the spin-glass compound $(Li_xV_{1-x})_3BO_5$ ($x \approx 0.40$ and 0.33)," Phys. Rev. B **76**, 054452 (2007).

[8] M. Frachet, I. Vinograd, R. Zhou, S. Benhabib, S. Wu, H. Mayaffre, S. Krämer, S. K. Ramakrishna, A. P. Reyes, J. Debray, T. Kurosawa, N. Momono, M. Oda, S. Komiya, S. Ono, M. Horio, J. Chang, C. Proust, D. LeBoeuf, and M.-H. Julien, "Hidden magnetism at the pseudogap critical point of a cuprate superconductor," Nat. Phys. **16**, 1064 (2020).

[9] Z. Zeng, X. Ma, S. Wu, H.-F. Li, Z. Tao, X. Lu, X.-h. Chen, J.-X. Mi, S.-J. Song, G.-H. Cao, G. Che, K. Li, G. Li, H. Luo, Z. Y. Meng, and S. Li, "Possible Dirac quantum spin liquid in the kagome quantum antiferromagnet $YCu_3(OH)_6Br_2[Br_x(OH)_{1-x}]$," Phys. Rev. B **105**, L121109 (2022).

[10] Y. Li, D. Adroja, P. K. Biswas, P. J. Baker, Q. Zhang, J. Liu, A. A. Tsirlin, P. Gegenwart, and Q. Zhang, "Muon spin relaxation evidence for the U(1) quantum spin-liquid ground state in the triangular antiferromagnet $YbMgGaO_4$," Phys. Rev. Lett. **117**, 097201 (2016).

[11] T. Itou, A. Oyamada, S. Maegawa, M. Tamura, and R. Kato, "Quantum spin liquid in the spin-1/2 triangular antiferromagnet $EtMe_3Sb[Pd(dmit)_2]_2$," Phys. Rev. B **77**, 104413 (2008).

[12] S. Lee, C. H. Lee, A. Berlie, A. D. Hillier, D. T. Adroja, R. Zhong, R. J. Cava, Z. H. Jang, and K.-Y. Choi, "Temporal and field evolution of spin excitations in the disorder-free triangular antiferromagnet $Na_2BaCo(PO_4)_2$," Phys. Rev. B **103**, 024413 (2021).

[13] P. Khuntia, F. Bert, P. Mendels, B. Koteswararao, A. V. Mahajan, M. Baenitz, F. C. Chou, C. Baines, A. Amato, and Y. Furukawa, "Spin liquid state in the 3D frustrated antiferromagnet $PbCuTe_2O_6$: NMR and muon spin relaxation studies," Phys. Rev. Lett. **116**, 107203 (2016).

[14] M. Fu, T. Imai, T.-H. Han, and Y. S. Lee, "Evidence for a gapped spin-liquid ground state in a kagome Heisenberg antiferromagnet," Science **350**, 655–658 (2015).

[15] Y. Shimizu, K. Miyagawa, K. Kanoda, M. Maesato, and G. Saito, "Emergence of inhomogeneous moments from spin liquid in the triangular-lattice Mott insulator $\kappa$-$(ET)_2Cu_2(CN)_3$," Phys. Rev. B **73**, 140407 (2006).

[16] J. A. Quilliam, F. Bert, A. Manseau, C. Darie, C. Guillot-Deudon, C. Payen, C. Baines, A. Amato, and P. Mendels, "Gapless quantum spin liquid ground state in the spin-1 antiferromagnet 6HB-$Ba_3NiSb_2O_9$," Phys. Rev. B **93**, 214432 (2016).
